# Supplementary material for: Molecular-scale substrate anisotropy and crowding drive long-range nematic order of cell monolayers
Source: arXiv:2210.13425 ancillary file (2022-10-24)
Supplement: Supplementary file 1 [file SI.pdf]

# Supplementary Materials for

## Molecular-scale substrate anisotropy and crowding drive long-range nematic order of cell monolayers


Yimin Luo[1,2], Mengyang Gu[3], Minwook Park[4], Xinyi Fang[3], Younghoon Kwon[2], Juan Manuel Urueña[5], Javier Read de Alaniz[4], Matthew E. Helgeson[1], M. Cristina Marchetti[6], and Megan T. Valentine[2,*]

[1]Department of Chemical Engineering, University of California, Santa Barbara, CA 93116
[2]Department of Mechanical Engineering, University of California, Santa Barbara, CA 93116
[3]Department of Statistics and Applied Probability, University of California, Santa Barbara, CA 93116
[4]Department of Chemistry and Biochemistry, University of California, Santa Barbara, CA 93116
[5]BioPACIFIC MIP, California NanoSystems Institute, University of California, Santa Barbara, CA 93116
[6]Department of Physics, University of California, Santa Barbara, CA 93116
[*]Corresponding author. Email: valentine@engineering.ucsb.edu



October 23, 2022


**This PDF file includes:**
Supplementary Text
Figs. S1 to S16
References (1 to 8)

**Other Supplementary materials for this manuscript include the following:**
Movies S1 to S5

The text portion is organized as follows: In Section 1, we illustrate the technical procedures to extract orientation, position and velocity from video sequences of live cell imaging. We first present the procedure to extract the position from the fluorescence channel associated with the cell nucleus in Section Note 1.1, and verify that the cell bodies are aligned with their nuclei in Section Note 1.2. The procedures to link the position across frames are discussed in Section Note 1.3.

In Section 2, we first present an analysis of the cell-cell order parameter in Section Note 2.1. This is related to both the cell-substrate order parameter shown in the main text and the orientational correlation functions, for which we show detailed fitting procedure in Section Note 2.2 to extract the correlation lengths and power-law exponents. A similar spatially-dependent correlation based on the velocity is the pair velocity correlation, shown in Section Note 2.3. Individual cells tend to move in a back and forth fashion, thus

we determine the average time for cells to switch their direction of movement in Section Note 2.4. We evaluate how the variance of the order parameter changes with box size in Section Note 2.5. We also show that, similar to other active systems, the cell number fluctuations grow faster than the system size in Section Note 2.6.

In Section 3, we provide details on the characterizations of the LCE substrate. Information on the materials is presented in Section Note 3.1. The details of LCE fabrication are presented in Section Note 3.2. To determine molecular order, scattering analysis is presented in Section Note 3.3. Mechanical testing is presented in Section Note 3.4, and surface characterizations are presented in Section Note 3.5.

In Section 4, we provide additional details on cell treatments and imaging. Cell handling protocols are presented in Section Note 4.1, imaging and image reconstruction are illustrated in Section Note 4.2, cell fixing procedures are described in Section Note 4.3, and the focal adhesion inhibitor treatment of the cells is shown in Section Note 4.4.

# Note 1 Position, orientation and velocity extraction

## Note 1.1 Ellipse fitting of the nuclei with a custom algorithm

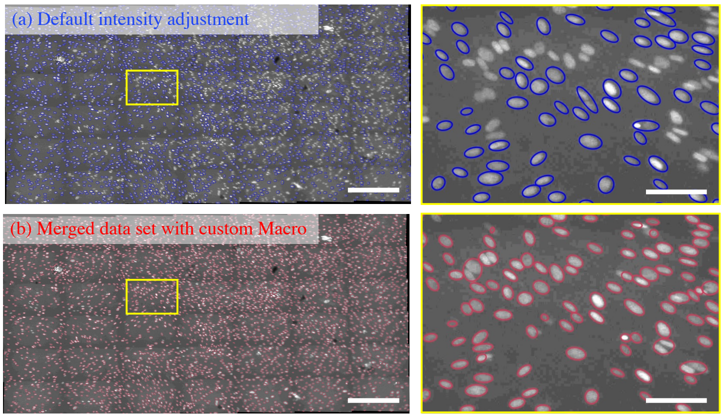


**Fig. S1**: Overlays of ellipses defected from the same image of the nucleus channel, threshold using the default brightness & contrast adjustment of FIJI on the top row, and using our standard, custom Macro adjustment and merging algorithm on the bottom row. The scale bars are 500 $\mu$m to the left, and 100 $\mu$m in the zoomed-in view to the right. (Note the apparent grid in is a result of slightly uneven illumination from 50% aperture opening and subsequent stitching).

The orientations of the cell nuclei were extracted using FIJI. In detail, the DAPI channel which represented the dyed nuclei was first split from the stack. The orientation of the nuclei was obtained by first converting the image to binary using a threshold determined by a custom Macro. Thereafter, the built-in 'analyze particle' function was used to determine the x, y positions, major and minor axes, and orientation ($\theta_i$, with respect to the horizontal) of the ellipses. The plug-in ROI manager was used to record the frame at which the ellipse was detected and manage the data outputs. Note that FIJI had a

default brightness and contrast adjustment function that evenly spreads the intensities over the full scale. As we were searching for a standard way of processing all images, we found that this adjustment followed by converting the image to binary, did not capture all of the cells, motivating the need for a custom Macro. We compare the performance of the two in Fig. S1. We found that our analysis scheme provides a $\sim$ 10-30% improvement when compared to ellipse detection using the built-in FIJI intensity adjustment algorithm (Fig. S1).

A combined csv file consisting of ellipsoid information with corresponding frame numbers was saved for post processing in MATLAB. An in-house code was written, to split the csv files by frame number, and then to compute the total number of cells per frame $N$ and cell-substrate order parameter $S_{cs}$ using Eq. (1) from the main text for each frame. Density $\rho$ was computed by dividing $N$ by the imaging area.

## Note 1.2 Verification of the alignment of cell body and nucleus orientations

To verify that the cell nucleus orientation was highly correlated with the orientation of the cell body, the orientation of the cell body was obtained by a similar ellipse fitting procedure, but now using data from the CellTracker channel, to obtain $\theta_B$, major and minor axis of the ellipse, and x, y positions for each cell (Fig S2a). Thereafter, $\theta_B$ and $\theta$ are paired with each other by finding the closest centroid positions amongst the other data set.

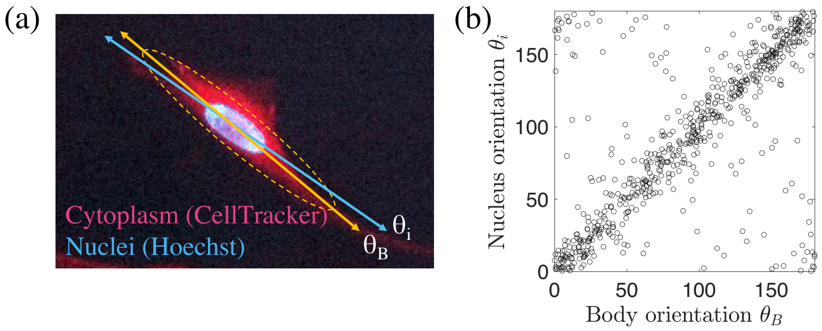


**Fig. S2**: (a) Schematic that shows the orientation of the nucelus $\theta_i$ versus that of the cell body $\theta_B$, (b) A scattering plot (in degrees) tallied from well-separated cells showing both angles are highly correlated or off by 180.

Since the body orientation and nucleus orientation both have head-tail symmetry, so does their difference, we thus computed the correlation coefficient between the cell body and its nucleus by:

$$C_{\text{nucleus-body}} = \langle 2\cos^2(\theta_B - \theta_i) - 1 \rangle, \tag{S1}$$

where the averaging was performed for $>$ 1000 cells, using frames where cells are reasonably well-separated to avoid complications associated with erroneous segmentation. We found that cell body orientation is highly correlated with its nucleus: $C_{\text{nucleus-body}} = 0.81$.

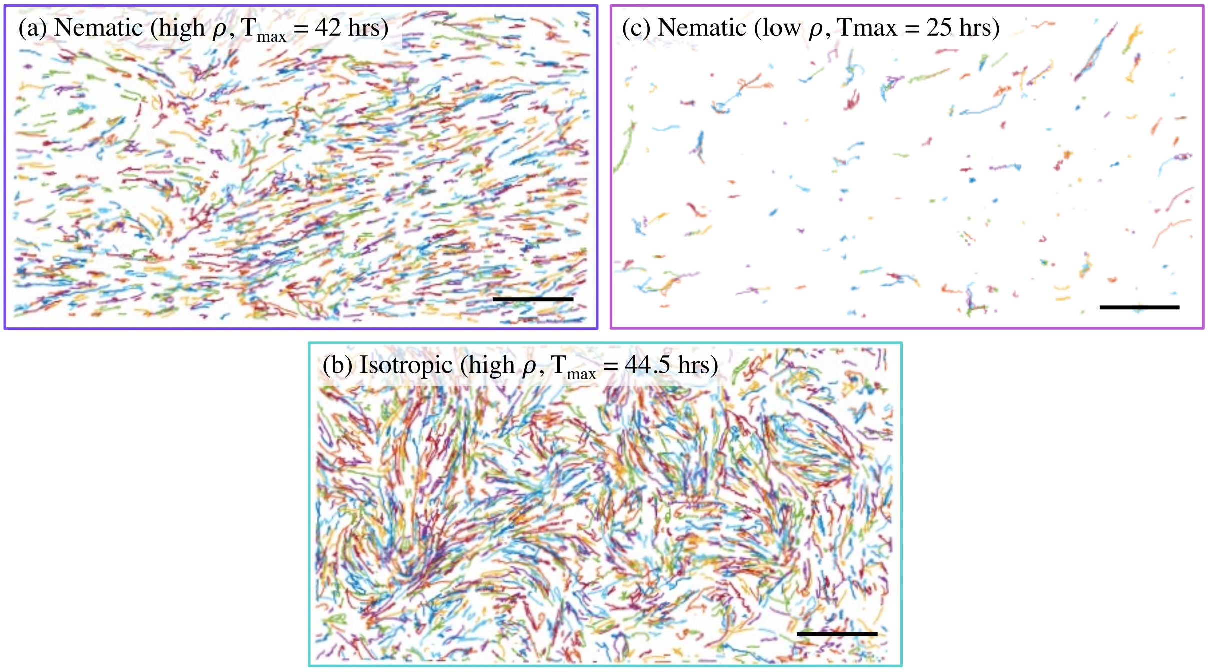


**Fig. S3**: Cell trajectories over time under different conditions as labeled. Different colors denote distinct trajectories. Several representative fields of view are shown: (a) is visualized at 20% original density, (b) at 50% and (c) at 100% for clarity. Only trajectories tracked for over 20 time steps are shown here. The scale bars are 500 $\mu$m.

## Note 1.3 Cell trajectory and velocity

The cell positions were next linked into trajectories using the FIJI plug-in TrackMate, where every nucleus is assigned a unique identification (TRACK ID) number to generate a csv file for post-processing in R and MATLAB; typical trajectories are shown in Fig. S3. This generates a new file, different from detecting centers by fitting ellipses. Thus, it was necessary to merge these two files to have both trajectory and ellipse information. This is done by matching ($x_i$,$y_i$) from both ellipse fitting and TrackMate by proximity and assign them the same TRACK ID.

Velocity was computed by first matching the entries in the csv file that are of the same TRACK ID over subsequent frames, then dividing the displacement over time intervals as follows: $v_x = \frac{x(t+\Delta t)-x(t)}{\Delta t}$, and similarly for $v_y$, using a custom R-algorithm. Note that in this context we use the term "velocity" loosely to denote the displacements from frame to frame, divided by the time interval. Finally, the speed was computed by $|v| = \sqrt{|v_x|^2 + |v_y|^2}$. We find through later analysis that cells travel back and forth with some randomness. However, as we will see, the notation is still useful in subsequent calculations of various quantities. Ultimately, the following standard format is adopted across all videos, containing the following columns: TRACK ID ($i$), FRAME ($t$), x position ($x_i$), y position ($y_i$), Major axis ($a$), Minor axis ($b$), Cell orientation ($\theta_i$), velocity x-component ($v_x$), velocity x-component ($v_y$), and vel angle ($\beta_i$).

## Note 2 Variable interpretation

### Note 2.1 The cell-cell order parameter $S_{cc}$

Another quantity often calculated to evaluate ordering is the cell-cell order parameter $S_{cc}$ :

$$S_{cc} = \langle 2\cos^2\theta_{ij} - 1\rangle \tag{S2}$$

where the averaging was performed over all cells included in an area. It computes the average order parameter over all pairs of cells located within an area, whereas $S_{sc}$ (Eq.(1) in the main text) computes the deviation with respect to a particular direction, i.e. the substrate orientation $\hat{\mathbf{e}}_x$. We find that $S_{cc}$ also grows with cell density $\rho$ (Fig. S4a) and that $S_{cc}$ varies similarly as $S_{cs}$ (Fig. S4b).

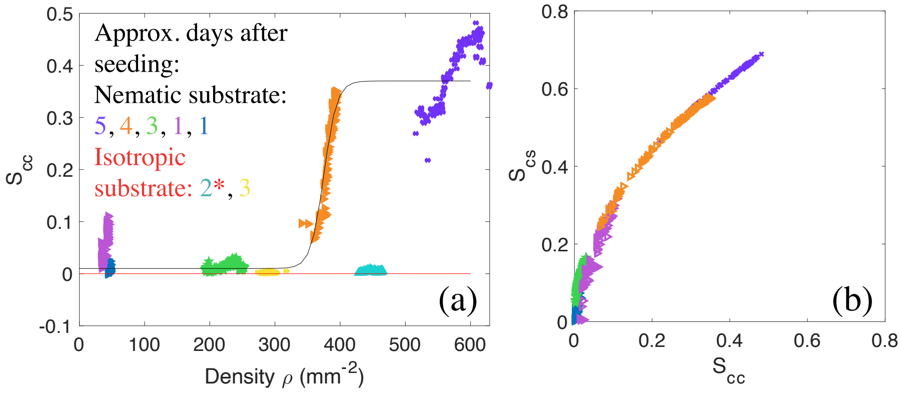


**Fig. S4**: (a) Cell-cell order parameter $S_{cc}$ for different cell densities, and how it varies with the cell-substrate order parameter $S_{sc}$ is shown in (b).

### Note 2.2 Pair orientation correlation function $C_{\theta\theta}$

In the main text, we compute the pair orientational correlation function:

$$C_{\theta\theta}(r) = \langle 2\cos^2\theta_{ij}(r) - 1\rangle. \tag{S3}$$

The pair orientation correlation functions are computed for all cell pairs separated by $r$, as shown in Fig. S5e, excluding self correlation ($i \neq j$). In practice, cell pairs are binned over the ring of radius $r$ ranging from 0 to 1000 $\mu$m in 10 $\mu$m increments and for ring width $dr = 10$ $\mu$m.

For cells moving on isotropic substrates at any density, or on nematic substrates when $\rho < \rho_c$: Correlation length $\xi_{\theta\theta}$ and normalizing coefficient $A_e$ are fit by taking the log on both sides of Eq. (3) from the main text:

$$\log\left(C_{\theta\theta}(r)\right) = \log A_e - \frac{r}{\xi_{\theta\theta}} \tag{S4}$$

and fit using a linear model (Fig. S5a,b,d). Plotting $C_{\theta\theta}$ versus $r$ on a log-lin plot will result in a line with slope is $-\frac{1}{\xi_{\theta\theta}}$.

For cells moving on nematic substrates when $\rho > \rho_c$: the coefficient $A_p$ and $\gamma$ are fit by taking the log on both sides of Eq. (4) from the main text:

$$\log\left(C_{\theta\theta}(r)\right) = \log A_p - \gamma \log(r) \tag{S5}$$

and fit using a linear model (Fig. S5c). Plotting $C_{\theta\theta}$ versus $r$ on a log-log plot will result in a linear plot where the slope is $-\gamma$.

We also considered a form that included the long-range order parameter $C_{\theta\theta}^{\infty}$:

$$C_{\theta\theta}(r) = A_p r^{-\gamma} + C_{\theta\theta}^{\infty} \tag{S6}$$

We first fit $C_{\theta\theta}(r)$ by using a separate set of parameters at each $\rho$ (at each time point), $\xi_{\theta\theta}(\rho)$, $A(\rho)$, stretched exponent$\gamma(\rho)$ and long-range ordering parameter $C_{\theta\theta}^{\infty}(\rho)$ fit using *lsqcurvefit* in MATLAB. The 95% confidence intervals were determined by *nlparci*, using the Jacobian matrix $J$, which is the partial derivative of each parameter of Eq. (S6) computed by *nlinfit*. However, fit value of $C_{\theta\theta}^{\infty}$ is nearly zero in all cases, indicating the variance in decreasing order can be accounted for by power-law alone. The parameters and fitting intervals are shown in Fig. S5.

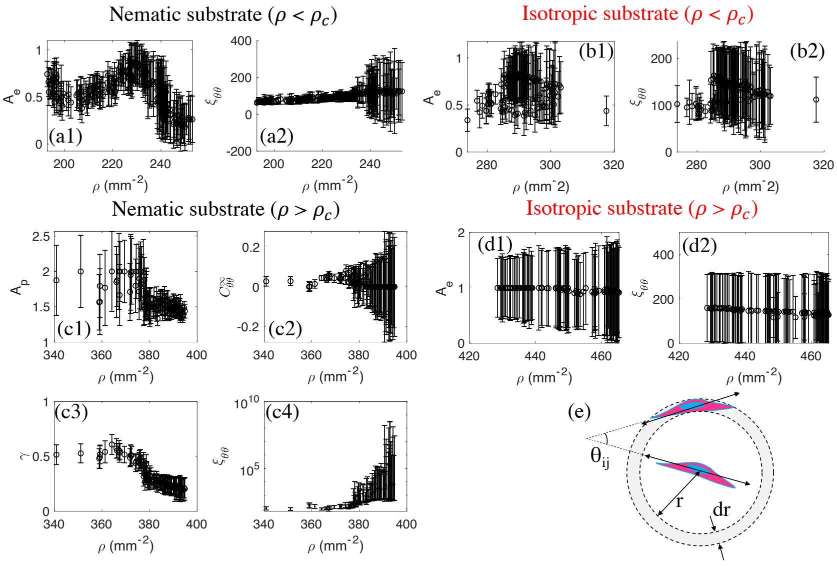


**Fig. S5**: (a-d) Fitting parameters for the orientational correlation functions used to analyze the motions of cells on nematic substrates for (a)(b) $\rho < \rho_c$ and (c)(d) $\rho > \rho_c$. (a)(b)(d) are fit following Eq.S4, and (c) is fit following Eq.S6.

We find that, initial fitting using all 4 parameters yield curves that fits the $C_{\theta\theta}$, but the parameters contain large error, potentially due to the covariance amongst all terms. It is very often the case that $\gamma$ is fixed for a given processes, and it appears to be the case as shown by Fig. S5c. So instead we fix $\gamma = 0.058 \pm 0.04$, and fit the rest of the parameters (Fig. 6). The log-log plots of Fig. 6a,b are shown in Fig. S5e,f.

## Note 2.3 The pair velocity correlation $C_{vv}(r)$

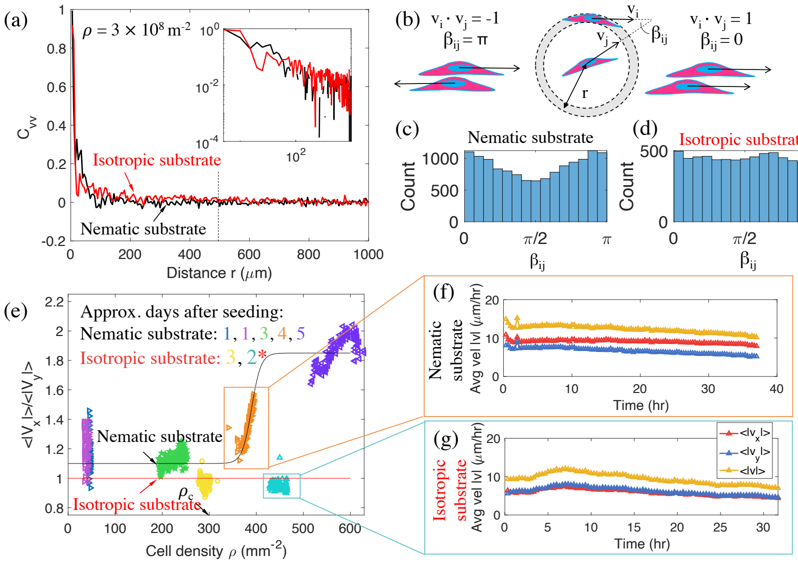

**Fig. S6**: Velocity correlations and anisotropy. Pair velocity correlations for cells moving on isotropic (red) and nematic (black) substrates. Inset: the same plot displayed on log-log axes. (b) Schematics showing that $C_{vv}$ is computed from binned values of separation distance between cell pair $ij$, where pairs with velocities aligned in anti-parallel fashion contributes $\hat{\mathbf{v}}_\mathbf{i} \cdot \hat{\mathbf{v}}_\mathbf{j}$ = -1 to the averaging, while co-traveling pairs contribute $\hat{\mathbf{v}}_\mathbf{i} \cdot \hat{\mathbf{v}}_\mathbf{j} = 1$. The distributions of $\beta_{ij}$, angle between velocity vectors, is shown in (c-d) for nematic and isotropic conditions, respectively at $r = 500$ $\mu$m (dotted line in (a)). Absolute velocity anisotropies are computed in (e), showing a significant increase in anisotropy for cells on nematic substrates at high density $\rho > \rho_c$. The time series of cell velocities and velocity components on isotropic and nematic substrates at similar densities are shown in (f) and (g). Data with the red asterisk denotes a run with a different initial seeding density.

We next computed the (polar) pair velocity correlation function:

$$C_{vv}(r) = \left\langle \frac{\vec{v}_i \cdot \vec{v}_j}{|\vec{v}_i||\vec{v}_j|} \right\rangle = \langle \hat{\mathbf{v}}_\mathbf{i} \cdot \hat{\mathbf{v}}_\mathbf{j} \rangle = \langle \cos \beta_{ij} \rangle, \tag{S7}$$

where $\hat{\mathbf{v}}_\mathbf{i}(t) = \frac{\vec{v}_i}{|\vec{v}_i|}$ denotes the unit velocity vector of cell $i$ at time $t$, $r$ is the center-to-center distance between cell $i$ and $j$ ($i \neq j$), $\beta_{ij}$ is the angle between the two velocity vectors [8, 5], and the averaging is performed over all cell pairs as before, with $dr = 10$ $\mu$m (Fig. S6a). $C_{vv} > 0$ means that the cells are following one another both moving in the same direction, whereas $C_{vv} < 0$ means that cells are moving towards one another from opposing directions (Fig. S6b).

For cells moving on either isotropic or nematic substrates, we found that the velocity correlation decays to zero rapidly for both conditions (Fig. S6a inset). In fact, we found that $C_{vv} = 0$ everywhere except within 1-2 cell widths for all $\rho$. However, further inspection of the distribution of angles $\beta_{ij}$ reveals a difference. For cells moving on either isotropic or nematic substrates, the distribution is bimodal for small $r$, indicating that cells show a preference to align with each other in either a parallel ($\beta_{ij} = 0$) or anti-parallel ($\beta_{ij} = \pi$) manner (Fig. S6b). We found that this bimodal distribution extends to only

to 100-200 $\mu$m on an isotropic substrate, comparable to the measured value of $\xi_{\theta\theta}$, while it persists to over 1000 $\mu$m on a nematic substrate, consistent with the cell monolayer having long-range order (Fig. S6c,d). Together, this provides strong evidence that steric interactions dominate the dynamics of cell organization in this weakly-interacting cell type.

We further related the cell-averaged velocity anisotropy, $\frac{\langle |v_x| \rangle}{\langle |v_y| \rangle}$ to $\rho$, and found that cells preferentially order along $\hat{\mathbf{e}}_x$ only for the nematic substrate, and only for $\rho > \rho_c$, due to coupling between cell pair orientation and velocity (Fig. S6e). While the average speeds of cells moving on both types of substrates were similar, there was a measurable increase in the $x$-component of the velocity (i.e., in the direction of nematic orientation) for cells moving on nematic substrates (Fig. S6f,g). This suggests that the multi-cell lanes that form at intermediate cell densities are composed of multiple single-cell files that can travel in parallel or antiparallel directions. While individual cells move back and forth and their motion is best characterized as nematic (Fig. S7a), their instantaneous direction is highly correlated with adjacent cells. As a result, the orientation of these bidirectional "highways" can be steered to align to a nematic LCE substrate.

## Note 2.4 The velocity auto correlation function (VAF)

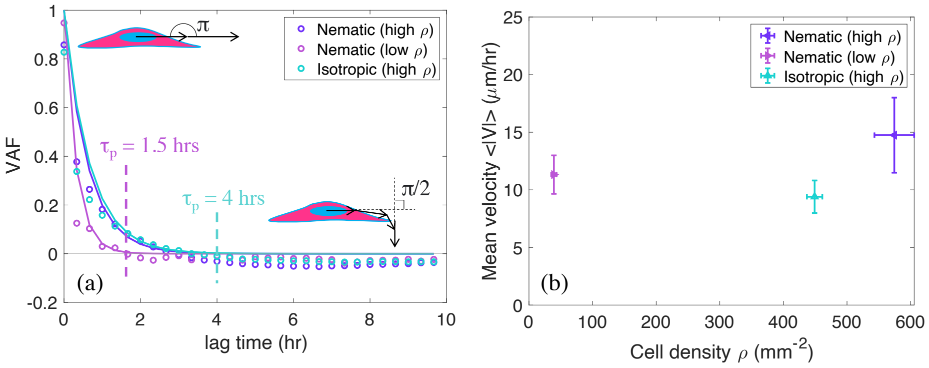


**Fig. S7**: (a) Velocity Autocorrelation Functions (VAF) as a function of lag time and (b) the mean velocity $|V|$ at different cell densities. The persistence time $\tau_p$, the lag time before a cell takes a $\pi/2$ turn was estimated from this plot to be about 1.5 hour for cells on cells at low density on a nematic substrate and about 4 hours for either substrates at high cell density.

To determine the characteristic timescales over which a single cell deviates from its original traveling direction (i.e. making a $\pi/2$-degree turn), we computed the velocity auto correlation function (VAF) from single-cell trajectories. This is done by tracking all entries in the above format with the same TRACK ID across different FRAME, and computing the inner product of instantaneous velocity angles $\beta$'s of a single cell at time $t$ and a later time $t + \Delta t$.

$$\text{VAF} = \langle \hat{\mathbf{v}}_\mathbf{i}(t + \Delta t) \cdot \hat{\mathbf{v}}_\mathbf{i}(t) \rangle \, , \tag{S8}$$

where the averaging was performed over all cells and all times $t$, where $\hat{\mathbf{v}}_{\mathbf{i}}$ is the unit vector of the velocity direction of cell $i$, $\Delta t$ represents the lag time. For each experiment, we computed the VAF for 30 $\Delta t$'s, ranging from 0 to 10 hours. Only trajectories that were tracked for at least 30 time steps are included in this calculation.

We find that the time it takes for cells to make a $\frac{\pi}{2}$ degree turn (going from VAF = 1 to VAF = 0) on average is roughly $\tau_p \approx 1.5$ hours at low $\rho$ and $\tau_p \approx 4$ hours for high $\rho$ (Fig. S7a). Considering the average velocity of $\sim 10$ $\mu$m/h, each cell travels an average distance $l \approx 30$ $\mu$m before turning around (= a $\pi$ degree turn), At higher $\rho$, this number stands at $\approx 80$ $\mu$m on an isotropic substrate, versus $\approx 120$ $\mu$m on a nematic substrate. Given that $l$ is significantly smaller or on the order of the body length of the cell ($\approx 100$ $\mu$m). The picture is consistent with one where the cell movement is nematic in nature, moving back and forth in place.

## Note 2.5 Effects of the box size

To investigate the effect of box size in determining the alignment parameters, we followed a procedure similar to bootstrapping with the full image (Fig. S8a), which had a size of 4mm $\times$ 2mm. We first sub-sampled boxes of a predetermined size $L_x \times L_y$, and found the number of cells $N$ and cell-substrate order parameter $S_{sc}$ within the box. Then we shifted the box by $dx$, to determine these quantities for a neighboring box with some overlap from the first box drawn. We repeated the process until the entire image area had been sampled. For instance, for $L_x = L_y = 300$ $\mu$m, and $d_x = d_y = 60$ $\mu$m (Fig. S8a), a total of $\sim$1750 boxes could be drawn, containing $N^i$ cells, with an order parameter $S^i_{sc}$, where the sample size was $i = 1,2,...$ 1750. We thus computed the average cell number and the corresponding average cell-substrate order parameters as: $\langle N \rangle = \frac{\sum N^i}{\sum i}$, and $\langle S_{sc} \rangle = \frac{\sum S^i_{sc}}{\sum i}$, and their standard deviations $\Delta N$ and $\Delta S_{sc}$, respectively.

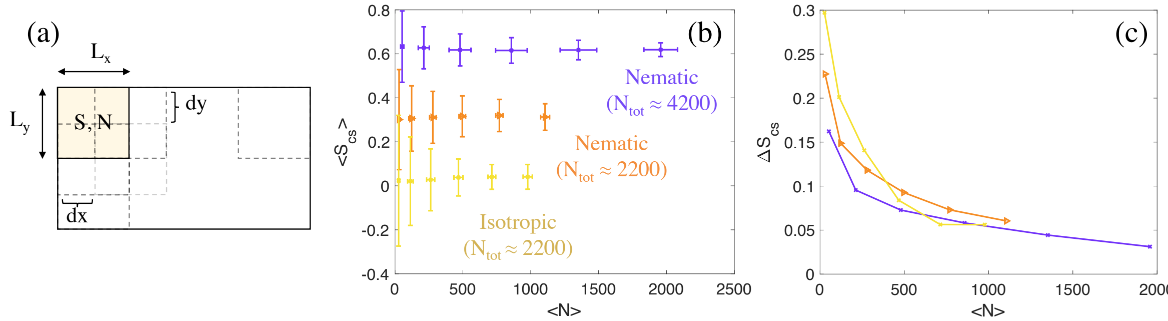


**Fig. S8**: Effects of the box size on the measurement of cell-substrate correlations. (a) Schematic of how the ensemble of $N$'s and $S_{sc}$'s within a box of size $L_x$ and $L_y$ were found. (b) Dependence of the mean value of $S_{sc}$ on the average number of cells $\langle N \rangle$ in each box of size $L_x \times L_y$. (c) Dependence of the variance of the order parameter $\Delta S_{cs}$ on the average number of cells $\langle N \rangle$.

Then we repeated this process with a new box size $L_x \times L_y$. For each box size, we computed the average order parameter $\langle S_{sc} \rangle$ and average cell number $\langle N \rangle$. As expected,

$\langle S_{sc}\rangle$ remained constant, no matter what box size $L_x \times L_y$ was chosen (Fig. S8b), since through repeated sampling, all order parameters are averaged over the full image (4mm $\times$ 2mm). However, the typical variance $\Delta S_{sc}$ was surprisingly large for small $\langle N\rangle$ (Fig. S8c). This suggests that when cell density was low or when the box size was small, resulting in fewer cells to calculate the $S_{sc}$, there might be an insufficient resolution to distinguish $S_{sc}$ measured between two substrates. This error in the $S_{cs}$ calculation appeared to only depend on the number of cells $\langle N\rangle$ averaged within a box, and not on whether the substrate was isotropic or nematic, or on the absolute cell density. This confirms that $S_{sc}$ is a pure statistical quantity, and $\Delta S_{sc}$ only depends on $\langle N\rangle$, this was the basis of how the uncertainty interval of $S_{sc}$ was assessed empirically in Fig. 3a in the main text, assuming $N = \langle N\rangle$. More rigorous derivation of how $\Delta N$ and $\Delta S_{sc}$ influence one another, is beyond the scope of this work.

## Note 2.6 Giant number fluctuations

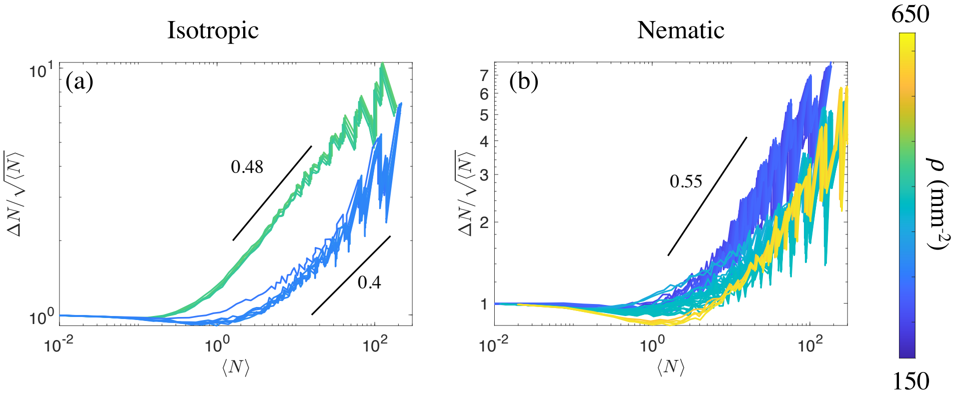


**Fig. S9**: Giant number fluctuations in the cellular density, color coded by density for (a) cells moving on isotropic substrates or (b) nematic substrates.

In an equilibrium system, we expect $\Delta N \propto \sqrt{\langle N\rangle}$, where $\Delta N$ denotes the standard deviation of particle number and $N$ denotes the averaged number of cells within each region. Active systems, on the other hand, exhibit giant number fluctuations (GNF) [3], where $\Delta N$ grows faster than $\sqrt{N}$ i.e. $\Delta N/\sqrt{\langle N\rangle} \sim \langle N\rangle^{\alpha}$ where $\alpha > 0$ [4]. To compute the mean and the variance, we following similar procedures as Sectioin Note 2.5. As expected, we observe GNF on both isotropic (Fig. S9a) and nematic substrates (Fig. S9b). Density fluctuation with the large $\alpha$ at lower $\rho$ likely facilitates the formation of locally dense and aligned domains such as those shown in Fig. 2c and e in the main text. $\alpha$ decreases for higher cell density, which can be attributed to motility arrest close to cell jamming [1].

# Note 3 Material characterization

## Note 3.1 Materials

Reactive monomers, diacrylate RM82 (1,4-Bis-[4-(6-acryloyloxyhexyloxy)benzoyloxy]-2-methylbenzene) and monoacrylate RM23 (4-[4-[6-Acryloxyhex-1-yl)oxyphenyl]carboxy-benzonitrile) were purchased from SYNTHON Chemicals GmbH & Co. KG and used without modification. RM82 and RM23 were mixed in 1:1 molar ratio (66:33 w/w), together with 1% photoinitiator DMPA (2,2-Dimethoxy-2-phenylacetophenone). The chemical structures of the compounds are shown in Fig. 1 in the main text.

## Note 3.2 LCE elastomer fabrication

Prior to film fabrication, the phase transition temperature from isotropic to nematic $T_{NI}$ of the RM82/RM23 mixture was determined by differential scanning calorimetry (DSC) using a TA Instruments Q2000 DSC with 50 position autosampler. The sample was first equilibrated at 0$^o$C. Then the release of heat from exothermic transitions was measured during a series of temperature ramps. Each cycle consisted of ramping at 10$^o$C/min to 120$^o$C, and after an isothermal hold for 1 min, cooling at 10$^o$C/min to 0$^o$C (Fig. S10). The resulting heat flow diagram is shown in Fig. S10 where the first large peak indicates the temperature of crystallization, and a smaller peak at 95$^o$C is the $T_{NI}$.

To make a nematic LCE film, the RM82/RM23 mixture was melted at 105$^o$C and introduced into a homemade sandwich chamber via capillarity. The chamber consisted of two poly-vinyl alcohol (MW = 9-10k, 80% hydrolyzed, Sigma-Aldrich) rubbed glass slides, separated by a 10 $\mu m$ spacer, which determined the film thickness. The temperature was lowered to below the isonematic transition temperature ($T_{NI} \sim 95$ $^o$C, found by DSC, Figure S1). As soon as the LC mixture acquired an aligned nematic state, it was illuminated using a handheld UV lamp (wavelength = 365 nm, 6W, Analytik Jena) for 20 minutes to completely crosslink the film. Thereafter, the chamber was immersed in Milli-Q water overnight to dissolve the PVA and release the film. The resulting anisotropic film could be visually checked between crossed polarizers (Fig. S10b-c). In Fig. S10b, the alignment of the molecules in the film was parallel to one of the polarizers, and the film appeared dark; in Fig. S10c, upon rotating the film by 45 degrees, the alignment of the molecules was not parallel to either of the polarizers, and the film appears bright.

To make an isotropic film, an identical procedure was followed except that the glass slides forming the chamber were not rubbed to impose uniform alignment and the UV illumination was carried out above the $T_{NI}$ at 105$^o$C. Then the film was released as before.

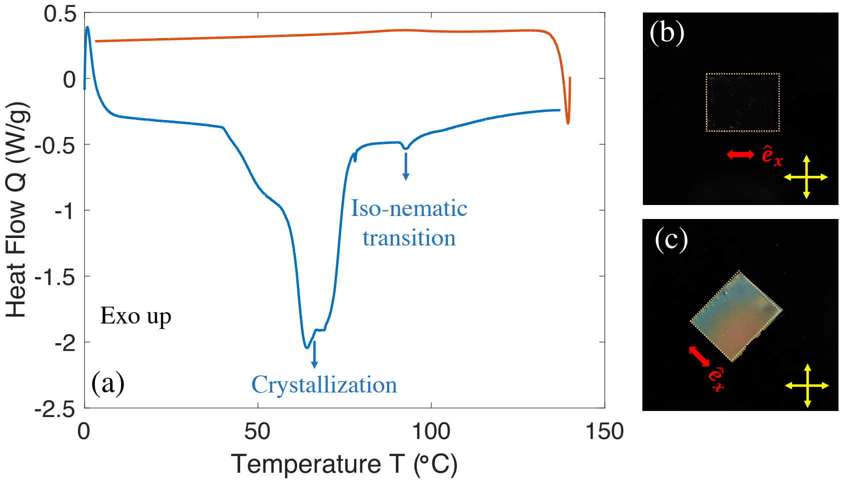


**Fig. S10**: (a) Differential scanning calorimetry to determine crystallization peak and iso-nematic transition temperature of the mixture. (b-c) Substrates were checked between crossed polarizers (yellow) to show alignments (along $\hat{\mathbf{n}}$). The outline of the substrate is denoted by the dashed line.

## Note 3.3 2D Small Angle X-ray Diffraction (WAXD)

To investigate the molecular alignment of the LCE films, two-dimensional (2D) wide-angle X-ray diffraction (WAXD) of the uniaxially oriented sample was obtained. The sample was illuminated with X-rays normal to the LCE alignment direction, using XENOCS Genix 50W X-ray microsource, and a focus size of 50 $\mu$m. A detailed schematic can be found in Fig. S11. The scattering intensity $I(\chi)$ is plotted against the azimuthal angle $\chi$ in Fig. S11b,d. $\chi_h$ is the half-width intensity, which is determined to be $\chi_h = 63$ ° for the nematic substrate and $\chi_h = 180$ ° for the isotropic substrate. We compute the order parameter (OP) using the following equation [7]:

$$\mathrm{OP} = (180^\circ - \chi_h) \times \frac{100^\circ}{180^\circ} \tag{S9}$$

Hence, the nematic substrate (Fig. S11a) has an order parameter of OP = 0.65, and the disordered substrate has an order parameter of OP = 0.

## Note 3.4 Dynamic Mechanical Analysis (DMA)

Dynamic mechanical testing was performed using oscillatory tensile loading using a TA Instruments DMA 850. Nematic films were prepared using the same methods as used in preparing the nematic substrates for the cell experiments (Fig. S13c). Two separate strips (8x10 mm) were prepared and clamped to measure the response in the two orthogonal directions: parallel and perpendicular to the LC alignment direction. The tests were performed at 0.5Hz and 0.01% strain. Time sweep data were collected for 3 minutes each in the two directions. The experiments were performed on both dry films in air at room temperature, and wet films that had been immersed in cell media at 37$^o$C. No discernable

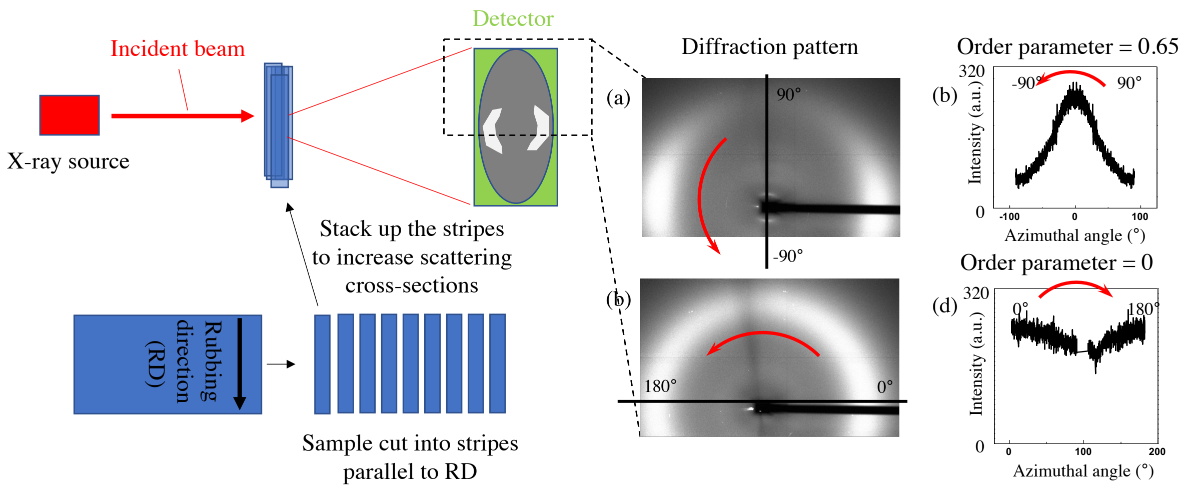


**Fig. S11**: Wide angle X-ray scattering to find the order parameter of the aligned substrate in (a-b), which has an order parameter of 0.65, and of the disordered substrate in (c-d), which has an order parameter of 0. The LCE elastomer was cut into stripes along the rubbing direction and stacked together to increase the scattering cross-sectional area.

differences in mechanical properties were found at different temperatures, between wet and dry conditions, or over time. Thus, the modulus values were reported as an average (bar plot, Fig. S12). For the isotropic substrate, there was no significant difference in the moduli along the two orthogonal directions, with measured values of 303 ± 83 MPa and 283 ± 10 MPa. By contrast, for the nematic substrate, the storage modulus along the direction parallel to the LC alignment direction was 3.5× higher than that along the perpendicular direction at 413 ± 27 MPa and 130 ± 4 MPa, respectively. Notably, the modulus of the isotropic substrate falls in between those along the two orthogonal directions of the nematic substrate.

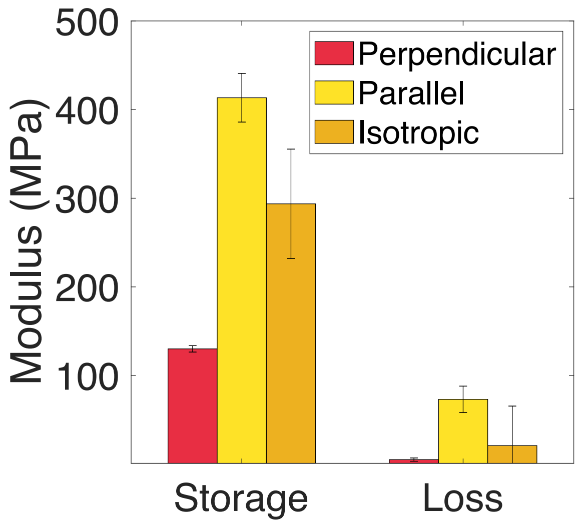


**Fig. S12**: Dynamic mechanical analysis performed on the nematic substrate shows that it also has anisotropic mechanical properties.

## Note 3.5 Surface roughness and topography characterization

Atomic force microscopy was performed with an Asylum MFP-3D Standard System to examine the surface roughness of the nematic LCE film. The scan area was set to be 5 $\mu$m x 5 $\mu$m (Fig. S13a) with 512 lines. The scan showed a root mean square roughness $R_q = 1.685$ nm. The surface was also examined using scanning electron microscopy using a FEI Inspect S Electron Scanning Microscope. A film was set to stand up on its side, fixed by carbon tapes, and imaged. The LCE substrate had a thickness of about 10 $\mu$m (Fig. S13b) and no significant surface topography features were observed.

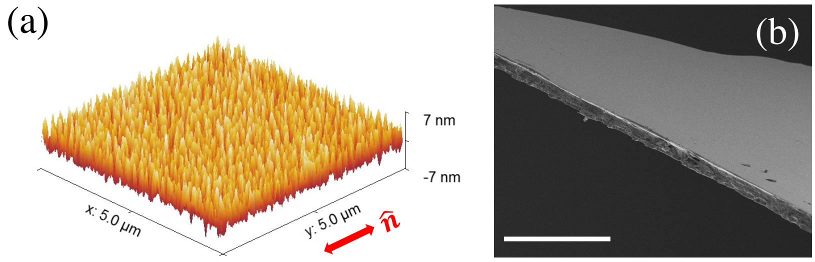


**Fig. S13**: Surface roughness characterization. (a) Surface roughness is determined by atomic force microscopy. (b) Scanning electron microscopy also shows that the surface is feature-less and the thickness is about 15 $\mu$m. The scale bar in (b) is 100 $\mu$m.

# Note 4 Cell handling and imaging

## Note 4.1 Cell culturing and seeding

Human dermal fibroblasts (hdFs, PCS-201-010) were purchased from American Type Culture Collection. Cells were cultured in cell media, consisting of Dulbeccos modified eagle medium (DMEM 1x + GlutaMAX, Gibco) supplemented with 10% fetal bovine serum (FBS, Gibco) and 1% Pen-Strep (Gibco) by volume, at 37$^o$C and 5% $CO_2$. Cells media were refreshed every other day and cells were sub-cultured whenever they reached 70-80% density (every 2-3 days), by lifting the cells with warmed 0.05% Trypsin, 0.53 mM EDTA (Corning) and gently tapping to dislodge them from the bottom. The lifted cells were pelleted at 1000 rpm, re-suspended in fresh media, and plated into a new culturing dish with a dilution factor of 3-4x. Passages 4 to 10 were used in experiments and no significantly different behaviors were observed as a function of passage or age. The doubling time of the hdFs is estimated to be ~50-60 hours in 10% serum from [6].

Given this doubling time, in order to observe a full range of cell densities (e.g., from 10% to 100% areal coverage), we would need to image cells for 6-8 days continuously if we plated at 10% and waited for proliferation to increase the density naturally. Unfortunately, even with optimized dye and illumination conditions, we found it very difficult to image living cells with fluorescent excitation beyond ~40 hours, due to the combined effects of cytotoxicity, bleaching, and sub-optimal media conditions. Instead, we varied the initial to control the cell density on the substrates, with proliferation playing a secondary role.

The film substrate was cleaned with isopropanol and glued using a coverslip sealant CoverGrip$^{TM}$ (Biotium) to the bottom of 35 mm petri dish with No. 1.5 coverslip bottom (MatTek Corporation). Care was taken to avoid wrinkles during film deposition. The glued substrate was pre-equilibrated in cell media. The equilibrating media also contained 2.5 $\mu$g/ml Amphotericin B fungicide (Gibco) to prevent fungal infection. Otherwise, the substrate was used without further functionalization. Previous literature [6, 2] found that hdF cells behave similarly on substrates whether or not they were coated with fibronectin, we also confirmed, by fixed cell imaging, that substrate coated with fibronectin induced similar cell alignment ($S_{cs} \approx 0.53$).

Cells were counted using a hemocytometer and seeded at volumetric density $\approx 2.5\times10^4$/mL, unless otherwise noted. Given the Petri dish diameter of 35 mm, this corresponds to an initial cell density of $\rho_s \approx 50$ mm$^{-2}$. Cell were cultured overnight to allow them to attach, then continuously cultured accompanied by media exchange for different periods of time (for a total of 1-5 days), until desirable confluency was reached.

## Note 4.2 Fluorescence staining and live cell imaging

Immediately prior to live cell imaging, cells were dyed while they were adhered to the substrate. Two dyes dissolved in Phosphate Buffered Saline (PBS) were used: CellTracker, which volumetrically labels the cytoplasm, at 500 nM, and Hoechst 33342, which labels the DNA within the nucleus, at 0.5 $\mu$g/mL. Cells were incubated with both dyes for 15 minutes, and then washed with PBS.

Imaging was performed using a Zeiss Axio Observer 7 microscope outfitted with a computer-controlled motorized sample stage, motorized auto-focus objectives, and Axiocam 702 monochromatic camera. Cells were maintained in the same cell culturing media during imaging, and the samples were placed in an incubation chamber which was maintained at 37$^o$C. A home-built chamber supplied a stream of humidified, 5% $CO_2$ in balanced air (Airgas) to maintain the pH of the imaging media. The cells were imaged using either a 10×/0.3NA air objective, at 2% power with LED illumination, 20 ms with DAPI filter (Ex = 358 nm, Em = 463 nm), and 50ms with Cy5 filter (Ex = 646 nm, Em = 664 nm), or with a 20×/0.8NA air objective, at 2% power, 5ms with DAPI filters, and 20ms with Cy5 filter. The average dwell time is about 2 seconds for each region of interest (ROI), with exposure time controlled by the shutter. The entire frame (42 ROIs) takes less than 2 minutes to scan. 2×2 binning was used to maximize the signal, thus the effective pixel sizes were 1.19 $\mu$m/pixel for 10× and 0.59 $\mu$m/pixel for 20×. When stitching together multiple tiles/fields-of-view, the imaging was carried out with an automated stage control, at a reduced speed, at 10% overlap and the field aperture was closed to 50% to avoid overexposure of the surrounding cells. A standard processing module in the Zeiss ZEN software was used to render a stitched image. A typical scan consisted of 42 tiles and took about 1 minute to complete. The cells were imaged at a rate of 1 stitched frame per 15-30 minutes and the entire imaging experiment lasted from 24-70 hours. The majority of the videos were taken at 20 min interval for 40 hours.

## Note 4.3 Cell fixation and immunofluorescence assay

To visualize either F-actin filaments or the fibronectin deposited by the hdF cells, cells were first fixed in 4% paraformaldehyde in PBS for 10 minutes, then rinsed 3× with PBS.

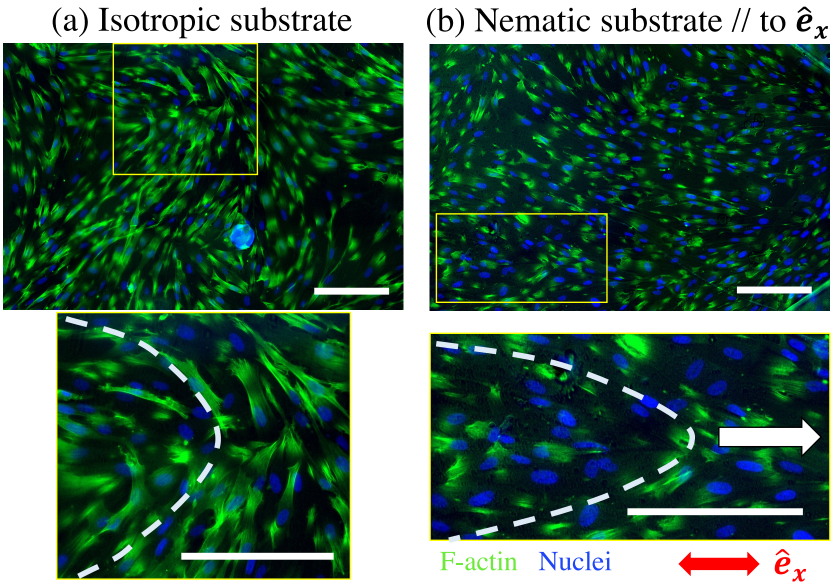


**Fig. S14**: (a-b) Overlay channels of nuclei (blue) and F-actin (green) for cells on (a) isotropic, (b) nematic substrates. Zoomed-in regions are shown around the $+\frac{1}{2}$ defects. The scale bars are 100 $\mu$m.

To visualize F-actin, the fixed cells were then stained by addition of Alexa Fluor 488 Phalloidin (Thermo Fisher) diluted 1:80 from stock (2.5 $\mu$l per 100 $\mu$l assay volume), which was allowed to incubate for 15 minutes at room temperature, and was then rinsed thrice with PBS. Fig. S14 shows staining of F-actin for cells on both isotropic and nematic substrates, and zoom-ins are shown in regions around the +1/2 defects.

To visualize fibronectin, the substrate-bound fibronectin deposited by the hdF cells was imaged (Fig. S15) using an immunofluorescence assay with anti-fibronectin monoclonal antibody (FN-3, eBioscience) conjugated with Alexa Fluor 488. Cells were first fixed in 4% paraformaldehyde in PBS for 10 minutes, then rinsed 3× with PBS. The fixed cells were then blocked using a 0.1% Bovine Serum Albumin (BSA, Sigma-Aldrich) in PBS solution at 4°C overnight, and then washed 3× with PBS. The anti-fibronectin antibody solution was then added at 0.1 mg/mL in 0.1% BSA, and incubated at room temperature for 45 min before washing 3× with PBS. The fixed cells were further stained with 1 $\mu$M CellTracker and 0.5 $\mu$g/mL Hoechst 33342 for 15 minutes, and washed 3× with PBS.

Fixed cells were imaged with the 20× objective with the following exposure time: 100ms with Cy5 filter, 20ms with DAPI filter and 50ms with GFP filter (Ex = 489 nm, Em = 509 nm) to capture either the F-actin or the FN-3 channel.

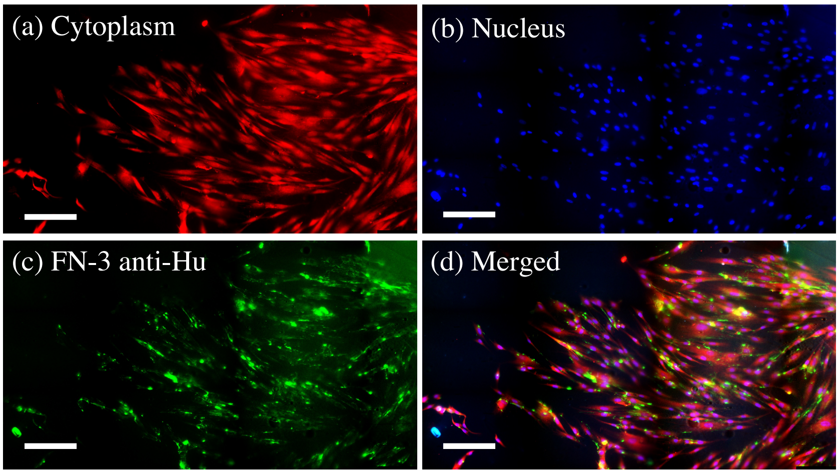


**Fig. S15**: Images demonstrating the results of immunofluorescence staining of fibronectin on fixed cells and their surrounding substrates. (a-c) Individual channels representing the fluorescence output of the cytoplasm, nucleus and the fibronectin antibody channels, and a single merged image in (d). Qualitatively, we observed that regions with cells have significantly more deposition of fibronectin. The scale bars are 200 $\mu$m.

## Note 4.4 Cell treatment with focal adhesion inhibitor (FAKi)

A control experiment was first carried out by seeding cells into 6-well dishes, at 200 $mm^{-2}$ and allowing them to attach overnight. The next day, cells were treated with 0.01, 0.1, 1, 10, 50, 100 $\mu$M of FAK inhibitor (1,2,4,5-Benzenetetramine tetrahydrochloride, Tocris Bioscience). The following day, we found that cells remain attached to the bottom at FAKi concentrations up to 1 $\mu$M, and thus 1 $\mu$M was used in the subsequent imaging experiment.

Cells were first cultured on a nematic substrate to $\sim$ 200 $mm^{-2}$, as before, without adding the inhibitor. Immediately before imaging, FAKi was added at 1 $\mu$M, and cells were imaged as before. Though FAKi was added at a low concentration, subsequent immunofluorescence staining (Fig. S16a,e) showed that the amount of stress fibers decreased for treated cells. The slow-down in cell proliferation also occurs much earlier, stabilizing at around 220 $mm^{-2}$, while the cell-substrate order parameter only increases to $\sim$ 0.28 (Fig. S16c), accompanied by a complete disappearance of velocity anisotropy. This result indicates that the alignment process is FAK-dependent.

# Movies

**Movie S1** The video shows a close-up view of moving patterns of four isolated cells on a nematic substrate that do not interact with each other. The cells' cytoplasm is dyed with Celltracker-Cy5, and their nuclei are dyed with Hoechst-blue, as described. Cells are observed to be moving back and forth in place, demonstrating their individual motion is nematic in nature. The video is played at 12000$\times$ real time and the scale bar is 50 $\mu$m.

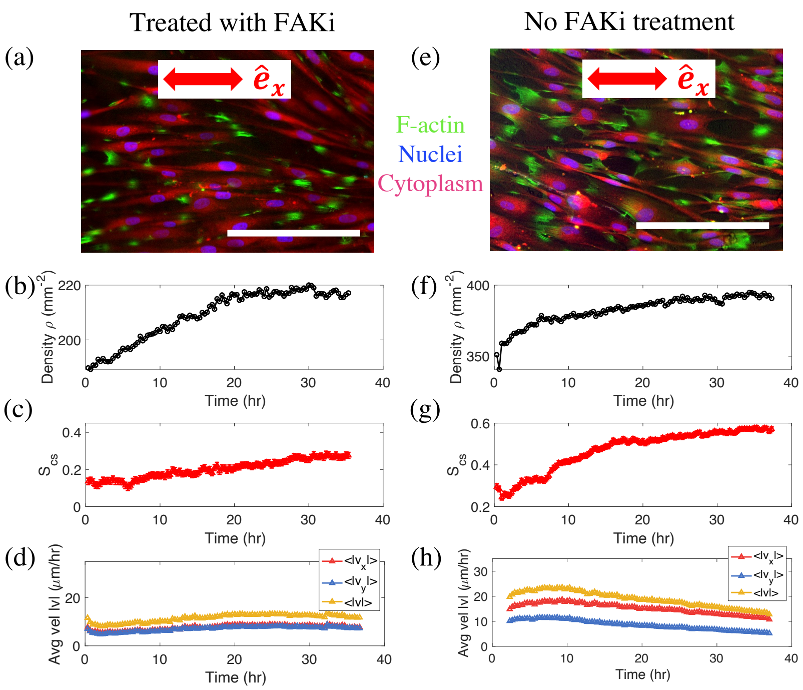


**Fig. S16**: Comparison of cells treated with focal adhesion kinase inhibitor (left) to those that have not been treated (right). Immunofluorescence staining of the actin, nuclei and cytoplasm are shown in (a-b) The scale bars are 100 $\mu$m in (a)(e). Cell density (b)(e), cell-substrate order parameter (c)(g) and average velocities (d)(h) were shown over time.

**Movie S2** The video shows the swirling motion of cells at an intermediate density ($\rho < \rho_c$) moving on a nematic substrate. Here, cells are forming streams and tracing out circles, but no global order has been established at this density. The video is played at 12000× real time and the scale bar is 100 $\mu$m.

**Movie S3** The video shows the evolution of a $+\frac{1}{2}$ (comet) defect moving with time as cells move on a nematic substrate along the LCE alignment direction. This video is played at 12000× real time and the scale bars are 100 $\mu$m.

**Movie S4** The video shows the evolution of a $+\frac{1}{2}$ (comet) defect moving with time as cells move on an isotropic substrate. This video is played at 12000× real time and the scale bars are 100 $\mu$m.

**Movie S5** The video shows the evolution of a $+\frac{1}{2}$ (comet) defect moving with time as cells move on a nematic substrate a perpendicular to the LCE alignment direction. This video is played at 12000× real time and the scale bars are 100 $\mu$m.

# References


[1] Thomas E Angelini, Edouard Hannezo, Xavier Trepat, Jeffrey J Fredberg, and David A Weitz. Cell migration driven by cooperative substrate deformation patterns.

*Phys. Rev. Lett.*, 104(16):168104, 2010.

[2] Greta Babakhanova, Jess Krieger, Bing-Xiang Li, Taras Turiv, Min-Ho Kim, and Oleg D Lavrentovich. Cell alignment by smectic liquid crystal elastomer coatings with nanogrooves. *Journal of Biomedical Materials Research Part A*, 108(5):1223–1230, 2020.

[3] Hugues Chaté, Francesco Ginelli, and Raúl Montagne. Simple model for active nematics: Quasi-long-range order and giant fluctuations. *Phys. Rev. Lett.*, 96(18):180602, 2006.

[4] Guillaume Duclos, Simon Garcia, HG Yevick, and P Silberzan. Perfect nematic order in confined monolayers of spindle-shaped cells. *Soft Matter*, 10(14):2346–2353, 2014.

[5] Camila Londono, M Jimena Loureiro, Benjamin Slater, Petra B Lücker, John Soleas, Suthamathy Sathananthan, J Stewart Aitchison, Alexandre J Kabla, and Alison P McGuigan. Nonautonomous contact guidance signaling during collective cell migration. *Proc. Natl. Acad. Sci. U.S.A.*, 111(5):1807–1812, 2014.

[6] Taras Turiv, Jess Krieger, Greta Babakhanova, Hao Yu, Sergij V Shiyanovskii, Qi-Huo Wei, Min-Ho Kim, and Oleg D Lavrentovich. Topology control of human fibroblast cells monolayer by liquid crystal elastomer. *Sci. Adv.*, 6(20):eaaz6485, 2020.

[7] Hyeong-Ho Yoon, Dae-Yoon Kim, Kwang-Un Jeong, and Suk-kyun Ahn. Surface aligned main-chain liquid crystalline elastomers: Tailored properties by the choice of amine chain extenders. *Macromolecules*, 51(3):1141–1149, 2018.

[8] Yu Zheng, Qihui Fan, Christopher Z Eddy, Xiaochen Wang, Bo Sun, Fangfu Ye, and Yang Jiao. Modeling multicellular dynamics regulated by extracellular-matrix-mediated mechanical communication via active particles with polarized effective attraction. *Phys. Rev. E*, 102(5):052409, 2020.
